# Supplementary material for: Theoretical Perspectives on Deep Learning Methods in Inverse Problems
Source: arXiv:2206.14373 source file (2023-01-30)
Supplement: Supplementary file 1 [file appendix.tex]

\section{Neural Networks and Deep Learning} \label{sec:neural_nets}

Here we provide a very brief introduction to neural networks and deep learning, primarily serving to set the relevant terminology used throughout the paper.  A detailed introduction to deep learning can be found in \cite{zhang2022dive}, among many others.

\begin{figure}
    \begin{centering}
        \includegraphics[width=0.85\columnwidth]{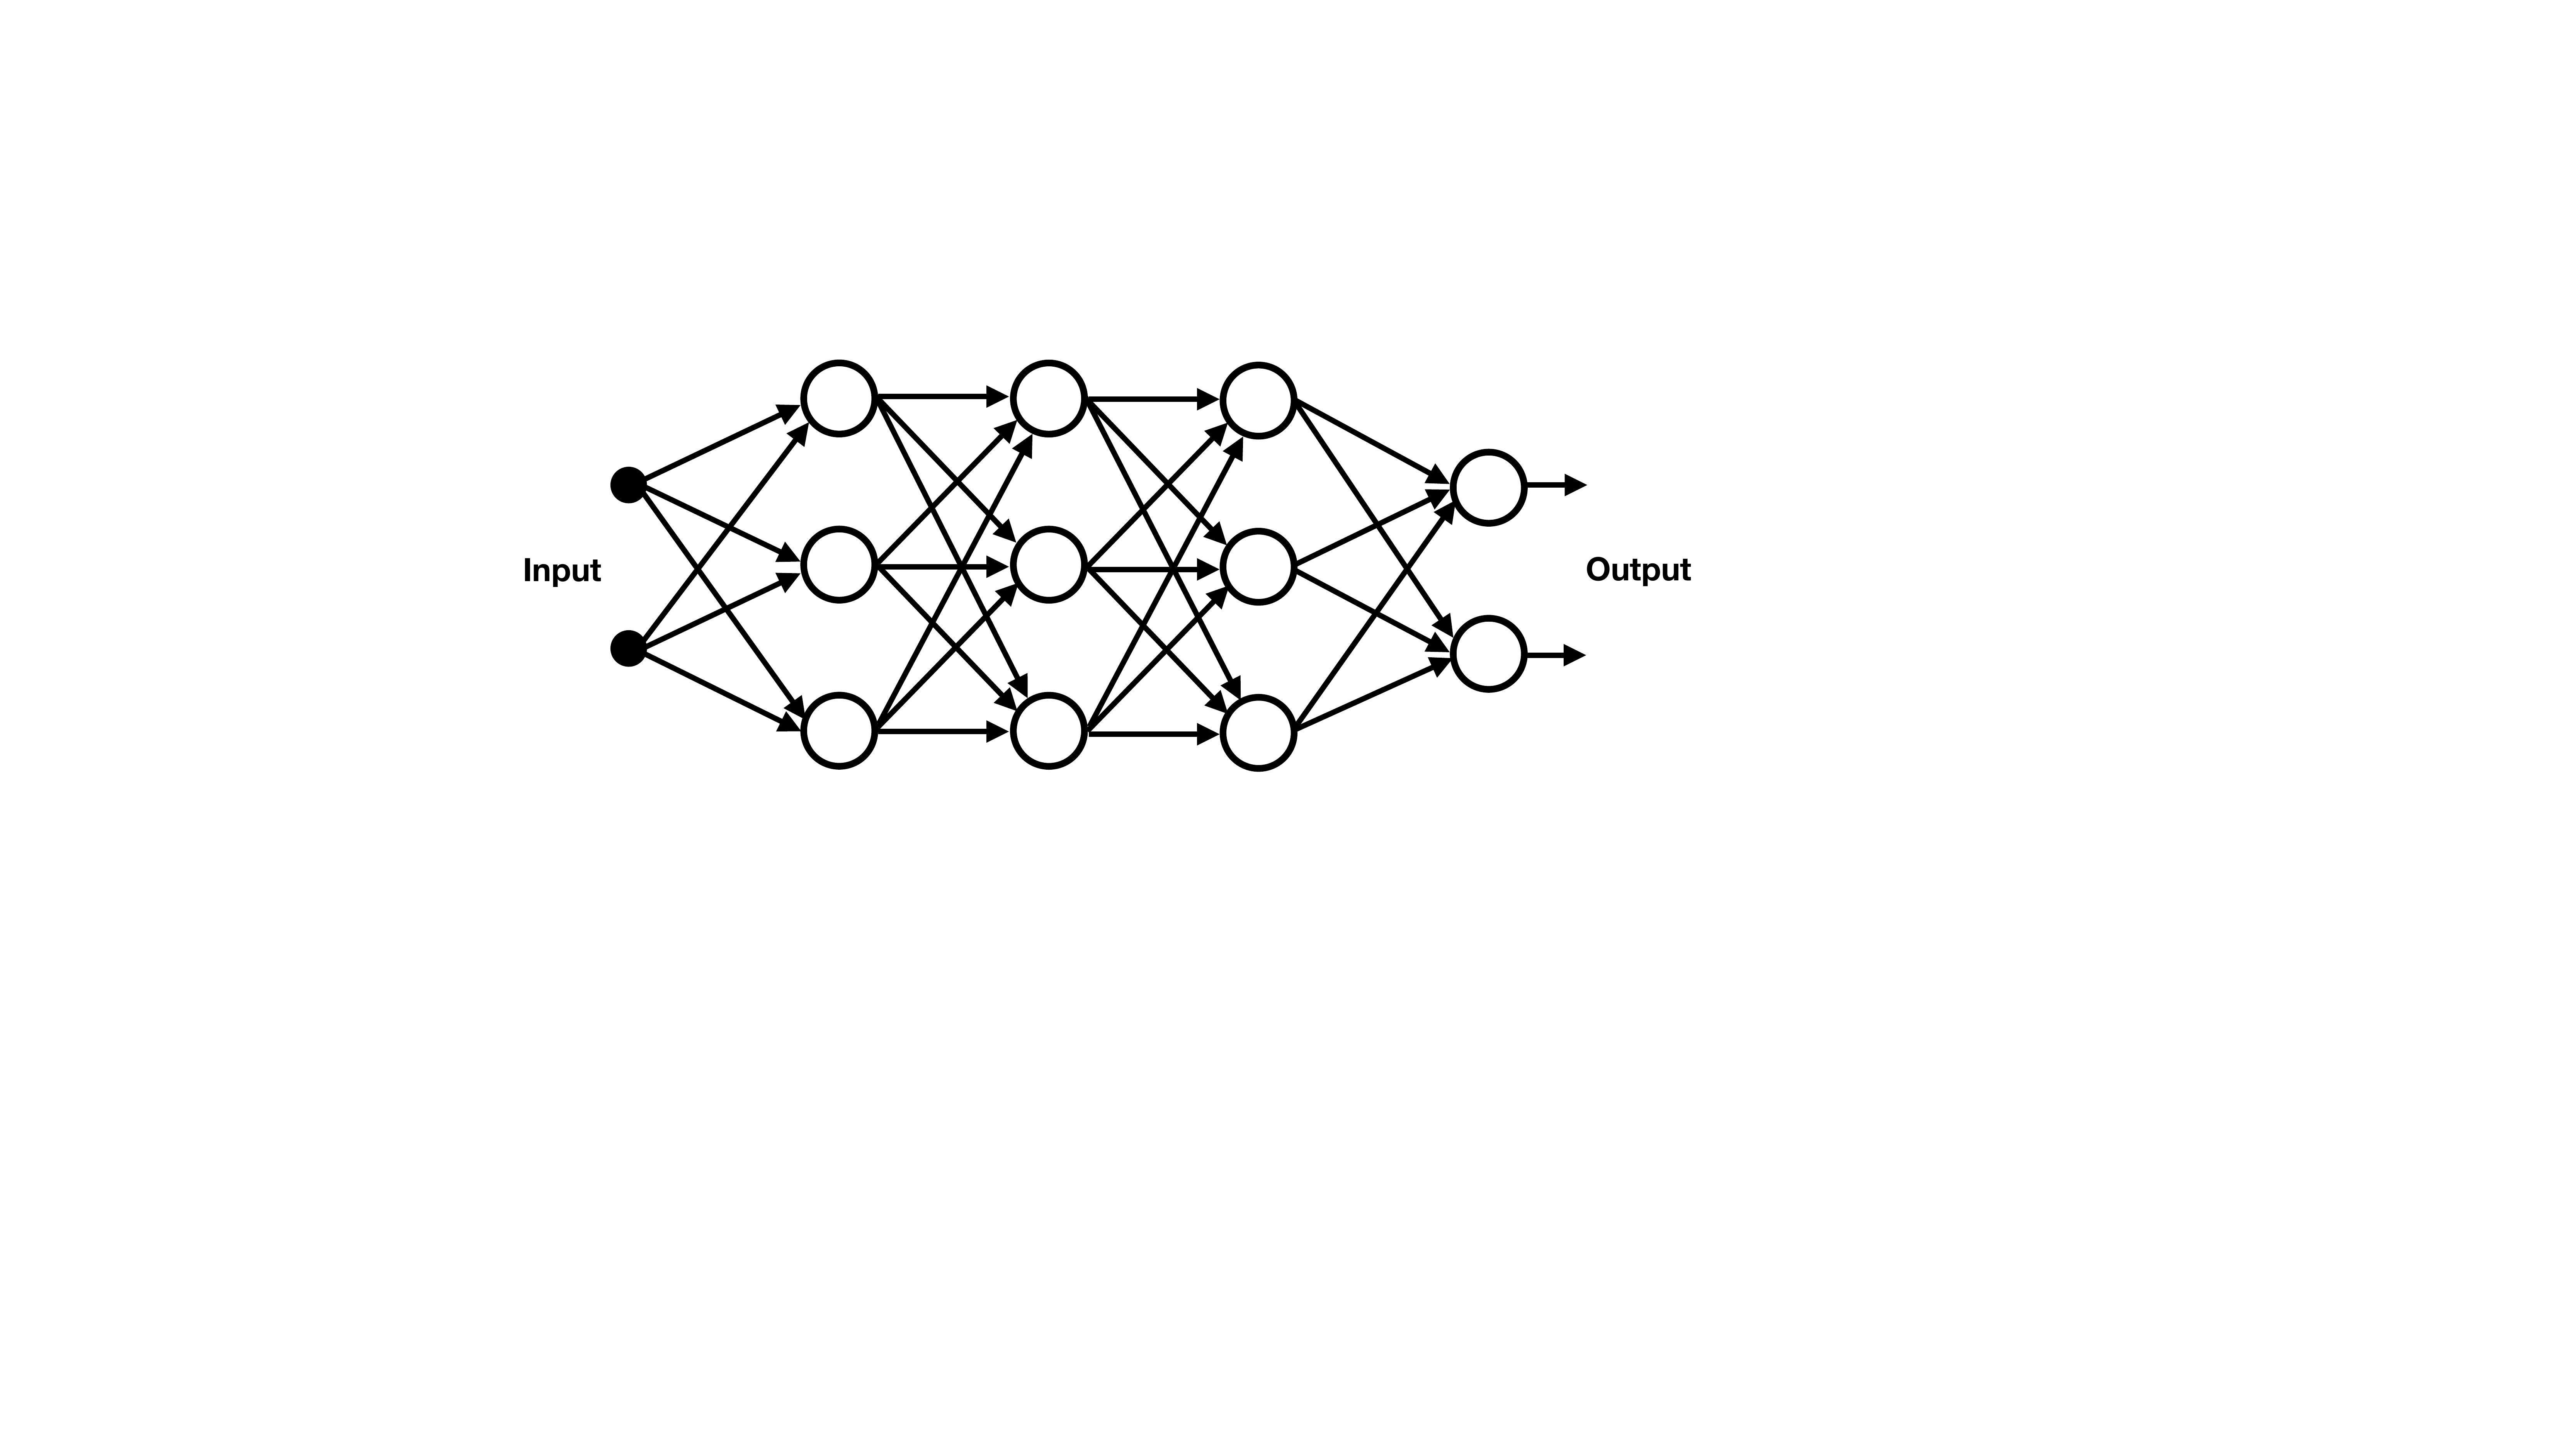}
        \par
    \end{centering}
    
    \caption{Simple example of a (fully-connected) neural network structure.  In this case, the width is 3 and the depth is 4.  \label{fig:nn}}
\end{figure}

A basic example of a neural network is depicted in Figure \ref{fig:nn}.  Each node is called a \emph{neuron}, and performs the simple operation of forming a weighted linear combination of its inputs (possibly plus a constant weight called the \emph{bias}), and then passing it through a non-linearity called the \emph{activation function}.  We primarily focus on the rectified linear unit (ReLU) activation function, $\relu(z) = \max\{0,z\}$, which is very widely used in practice.  
Each vector-to-vector map dictated by a collection of neurons is called a \emph{layer}, and key quantities of the neural network include the depth (number of layers) and width (maximum number of neurons in any layer).  The terminology \emph{deep learning} stems from frequently-observed benefits of having high depth, though this terminology is generally used quite loosely. 

Different choices of weights correspond to different overall functions, and the procedure of \emph{learning} consists of tuning the weights based on \emph{training data} in order to achieve some desired functionality.  This is typically done by performing an optimization procedure (e.g., gradient descent or a variant thereof) to minimize the empirical value of some \emph{loss function} (e.g., squared distance from the target), and the associated minimization problem is termed \emph{empirical risk minimization}.

Most introductory machine learning resources focus on the fundamental problems of classification and regression that dictate the desired functionality (e.g., let the input be an image, and seek an output that indicates whether or not the image contains a face).  In this survey, we are more interested in neural networks that output a \emph{signal}, such as an image.  For instance, when training a neural network to recover $\bx$ from $\by = \calA(\bx)$ with unknown $\calA(\cdot)$,\footnote{Not the be confused with classification/regression problems in which $y$ typically denotes the output.} the training data might consist of pairs $\{ (\by_i,\bx_i) \}_{i=1}^N$ with $\by_i = \calA(\bx_i)$, and the network weights might be tuned to minimize the loss function $\frac{1}{N}\sum_{i=1}^N \| \bx_i - \Psi(\by_i) \|^2$, where $\Psi(\cdot)$ is the overall neural network function from $\by$ to $\bx$.

The neural network in Figure \ref{fig:nn} is a very basic \emph{fully connected} network architecture.  For more complex scenarios, such networks are usually a poor choice, and one instead introduces certain kinds of structure into the layers, with the specific structure being dictated by the type of problem at hand.  In particular, we highlight the following:
\begin{itemize}
    \item \emph{Convolutional neural networks} (CNNs) consist of convolution layers, which use the same weights to map patches of the input to the output in a sliding window manner.  CNNs are particularly useful in imaging applications, where common features/objects may appear across different parts of the image.
    \item \emph{Recurrent neural networks} (RNNs) perform a common operation (typically sharing the same weights) repeatedly across the layers, and each layer may have its own separate input.  RNNs are particularly useful for handling sequential data, such as natural language text.
\end{itemize}
In theoretical analyses of deep learning, some of the most fundamental types of question that arise are as follows:
\begin{itemize}
    \item \emph{Representation}: What kinds of functions can neural networks represent for a given architecture?
    \item \emph{Generalization}: How well does the neural network perform on data that was not in the training set?
    \item \emph{Optimization}: What role does the optimization procedure play in finding a desirable solution?
\end{itemize}
Each of these are pertinent to deep learning methods in inverse problems, as we highlight throughout this survey.  Regarding generalization, we mention that poor generalization is typically attributed to \emph{overfitting} (i.e., finding spurious patterns in the training data), and is often resolved using some form of \emph{regularization} (e.g., adding a penalty term to the loss function, or stopping the optimization procedure early).
